# Supplementary material for: MMCR4NLP: Multilingual Multiway Corpora Repository for Natural Language Processing
Source: arXiv:1710.01025 source file (2019-02-14)
Supplement: Supplementary file 1 [file additional.tex]

% Please add the following required packages to your document preamble:
% \usepackage{graphicx}
\begin{table}[]
\begin{center}
\setlength{\tabcolsep}{.2em}
\begin{tabular}{|c|c|c|c|c|c|c|}
\hline
Language                                                            & Ar    & Fr    & Es    & Zh & Ru    & En    \\ \hline
\begin{tabular}[c]{@{}c@{}}Line\\ Count\end{tabular}                & \multicolumn{6}{c|}{11.36}                 \\ \hline
\begin{tabular}[c]{@{}c@{}}Word\\ Count\end{tabular}                & 262.7 & 339.4 & 350.1 & -  & 273.2 & 294.4 \\ \hline
\begin{tabular}[c]{@{}c@{}}Unique \\ Word\\ Count\end{tabular}      & 2.47  & 1.48  & 1.59  & -  & 2.24  & 1.64  \\ \hline
\begin{tabular}[c]{@{}c@{}}Average\\ Sentence\\ Length\end{tabular} & 23    & 29    & 30    & -  & 24    & 25    \\ \hline
\end{tabular}
\caption{Corpora statistics for the United Nations 6 lingual corpus.}
\label{uncorpus}
\end{center}
\end{table}

\begin{table}[]
\centering
\resizebox{\textwidth}{!}{%
\begin{tabular}{|c|c|c|c|c|c|c|c|c|c|c|c|c|c|c|c|c|c|c|c|c|c|c|}
\hline
Language &  & Da & De & Es & Pt & It & Nl & Fr & Fi & Sv & En & Hu & Lt & Lv & Bg & El & Et & Ro & Sk & Sl & Cs & Pl \\ \hline
\multirow{2}{*}{\begin{tabular}[c]{@{}c@{}}Line\\ Count\end{tabular}} & 21-way & \multicolumn{21}{c|}{0.189} \\ \cline{2-23} 
 & 10-way & \multicolumn{10}{c|}{1.07} & \multicolumn{11}{c|}{-} \\ \hline
\multirow{2}{*}{\begin{tabular}[c]{@{}c@{}}Word\\ Count\end{tabular}} & 21-way & 4.66 & 4.79 & 5.40 & 5.15 & 4.91 & 5.23 & 5.36 & 3.44 & 4.57 & 5.07 & 4.16 & 3.76 & 3.92 & 4.76 & 5.12 & 3.62 & 5.02 & 4.22 & 4.24 & 4.21 & 4.24 \\ \cline{2-23} 
 & 10-way & 25.84 & 26.29 & 29.67 & 28.65 & 27.26 & 28.76 & 29.52 & 19.15 & 25.61 & 28.19 & \multicolumn{11}{c|}{-} \\ \hline
\multirow{2}{*}{\begin{tabular}[c]{@{}c@{}}Unique \\ Word Count\end{tabular}} & 21-way & 0.145 & 0.162 & 0.114 & 0.120 & 0.122 & 0.127 & 0.109 & 0.274 & 0.147 & 0.083 & 0.269 & 0.206 & 0.169 & 0.138 & 0.143 & 0.247 & 0.129 & 0.175 & 0.164 & 0.179 & 0.188 \\ \cline{2-23} 
 & 10-way & 0.462 & 0.473 & 0.311 & 0.326 & 0.334 & 0.375 & 0.307 & 0.856 & 0.463 & 0.228 & \multicolumn{11}{c|}{-} \\ \hline
\multirow{2}{*}{\begin{tabular}[c]{@{}c@{}}Avg Sent\\ Length\end{tabular}} & 21-way & 24 & 25 & 28 & 27 & 25 & 27 & 28 & 18 & 24 & 26 & 22 & 19 & 20 & 25 & 27 & 19 & 26 & 22 & 22 & 22 & 22 \\ \cline{2-23} 
 & 10-way & 24 & 24 & 27 & 26 & 25 & 26 & 27 & 17 & 23 & 26 & \multicolumn{11}{c|}{-} \\ \hline
\end{tabular}%
}
\caption{Corpora statistics for the Europarl 21 lingual corpus.}
\label{my-label}
\end{table}
